# Supplementary material for: On the possibility of metastable metallic hydrogen
Source: arXiv:1705.04900 ancillary file (2017-05-13)
Supplement: Supplementary file 1 [file supplementary_information.pdf]

# Supplementary Information for: On the possibility of metastable metallic hydrogen

Craig M. Tenney,[1] Keeper L. Sharkey,[1] and Jeffrey M. McMahon[1,*]

[1]*Department of Physics and Astronomy,*

*Washington State University, Pullman, Washington 99164, USA*

This Supplementary Information contains results (and discussion) that were referred to, or supports those presented in the main text. It is organized similarly. Note that the figures and tables follow the text.

# I. SUPPLEMENTAL RESULTS

## A. Body-Centered Tetragonal Structures

Lattice parameters for the body-centered tetragonal (BCT) structures of atomic metallic hydrogen are reported in Supplementary Table I.

## B. Structure Prediction

### *1. Phase Diagram*

The phase diagram (at 0 K) of the most stable candidate structures of metastable metallic hydrogen, below molecular dissociation, are shown in Supplementary Fig. 1. Consistent with, and supporting the results in the main text, the pressure range can be (qualitatively) divided into three regions (note the reverse presentation, relative to the main text):

(c) $<$ 200 GPa: the relative enthalpies sharply decrease, with a magnitude proportional to the number of atoms. This is consistent with the tendency towards the formation of molecules (more atoms can form more molecules); supported by further analysis below.

(b) 200–300 GPa: crossovers of enthalpy begin to appear. Considering also the results at higher pressures (below), this is consistent with a transition region, where the underlying potential-energy surface (PES) of hydrogen changes.

(a) $>$ 300 GPa: many crossovers occur, to the extent of that there is a lack of general trend. This is consistent with significant changes in the underlying PES; in particular, energy barriers between metallic phases now exist. Note that the structures found at 0 GPa are also (likely) no longer representative of metastable ones.

### 2. *Mixed Atomic/Molecular Structures*

The most stable candidate mixed atomic/molecular structures are shown in Supplementary Fig. 2. Their corresponding structural parameters are reported in Supplementary Table II.

As remarked in the main text (and reported explicitly in Supplementary Fig. 2), there is a greater proportion of molecules (to atoms), as the number of atoms increases.

### 3. *Atomic Structures*

Structural parameters for the structures shown in Fig. 4 in the main text are reported in Supplementary Table III.

It is interesting to compare these structures to those found in Ref. 1. Therein, the lowest-energy structures (also, nearly degenerate in energy) were shown to be obtained starting from and distorting the primitive hexagonal lattice. This leads to a two-parameter, continuous set. Contained within this are structures shown in Fig. 4 in the main text.

## C. Dynamic Stabilities

### 1. *Body-Centered Tetragonal Structures*

The phonon density of states $F(\omega)$ of the BCT $\beta$-Sn structure is shown in Supplementary Fig. 3. Even though this structure becomes the most stable (of the BCT ones) at and below 350 GPa (Fig. 2 in the main text), it is dynamically unstable. Similar to the behavior of the Cs-IV structure (Fig. 5 in the main text), the instability increases with decreasing pressure.

### 2. *Atomic (Candidate) Structures*

Figure 6 in the main text revealed peaks with small magnitudes in $F(\omega)$ of the candidate (atomic) structures (Fig. 4 in the main text), at very high imaginary frequencies. Further analysis confirms that these are not anomalous. In particular, geometry relaxations of supercells relax these structures to (completely) molecular ones. The resulting structures are shown in Supplementary Fig. 4. Their corresponding structural parameters are reported

in Supplementary Table IV.

It is interesting to note that Ref. 1 also found such low (magnitude) phonons with imaginary frequencies. These were rationalized therein as anomalous, as very small deformations between similar structures with very close energies (analogous to the situation here; see the above discussion). The above analysis does not support this, however.

$F(\omega)$ of the most stable candidate (atomic) structures at 200 GPa (just below the limit of stability of the BCT ones; see Fig. 5 and the corresponding discussion in the main text) are shown in Supplementary Fig. 5. Dynamic instabilities are apparent.

---

* jeffrey.mcmahon@wsu.edu

[1] E. G. Brovman, Y. Kagan, and A. Kholas, Journal of Experimental and Theoretical Physics **34**, 1300 (1972).

**FIGURES**

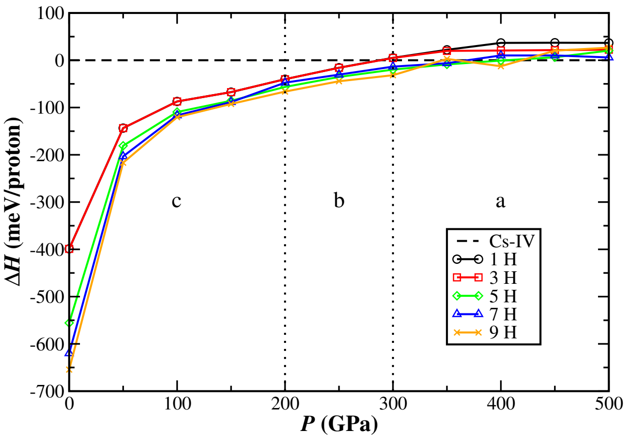


SUPPLEMENTARY FIG. 1. Phase diagram (at 0 K) of the most stable candidate structures of metastable metallic hydrogen, below molecular dissociation. Enthalpies $\Delta H$ are shown relative to Cs-IV, as a function of pressure $P$. Results are shown for searches with different numbers of atoms in the unit cell, up to 10. Three (qualitative) regions of stability are separated by dotted lines, and labeled a, b, c.

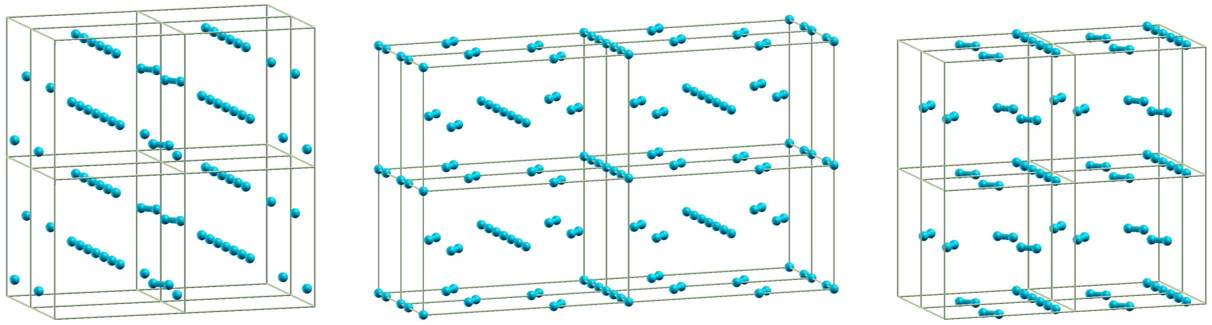

(a) C2 (5) [4:1] (b) C2/m (7) [3:4] (c) Pm (9) [1:2]

SUPPLEMENTARY FIG. 2. Most stable candidate mixed atomic/molecular structures, at 0 GPa. Structures are shown for searches with different numbers of atoms in the unit cell (specified in parenthesis). The atom:molecule ratios are specified in square brackets.

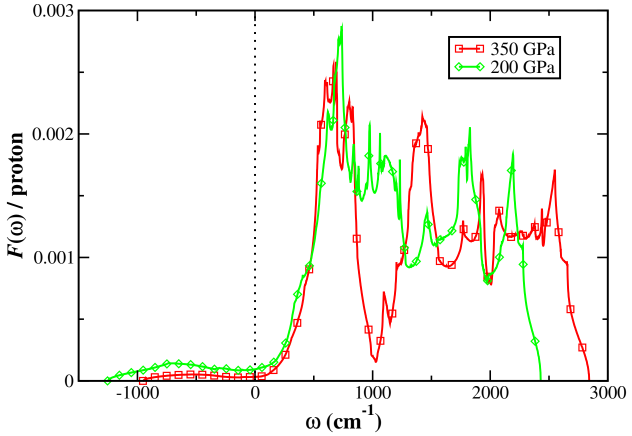


SUPPLEMENTARY FIG. 3. Phonon density of states $F(\omega)$ of the body-centered tetragonal (BCT) $\beta$-Sn structure of atomic metallic hydrogen. Two pressures are shown. A dotted line is used to separate the stable from unstable (imaginary) frequencies (shown as negative values).

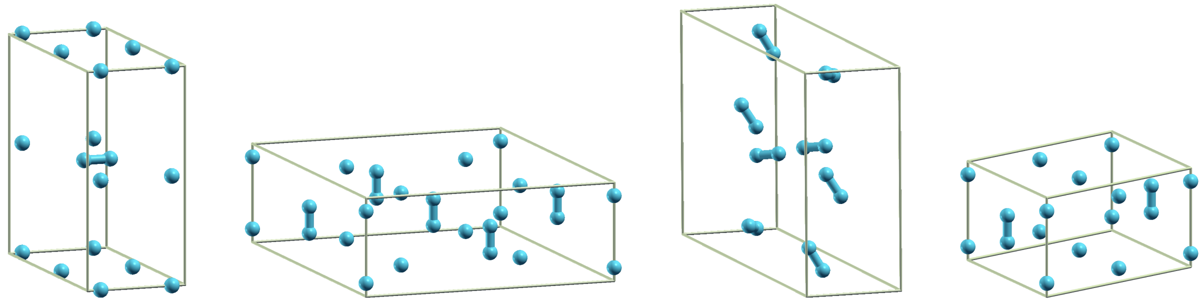

(a) Pmmm (Pmmm) (b) P2/m (Cmmm) (c) P$\bar{1}$ (Immm) (d) P2/m (P6/mmm)

SUPPLEMENTARY FIG. 4. Relaxed supercells (2×2×2) of the most stable candidate (atomic) structures (space groups specified in parenthesis), at 0 GPa (Fig. 4 in the main text). Their space groups are specified in the subcaptions. Note that atoms are paired across the unit cells in (a), (b), and (d).

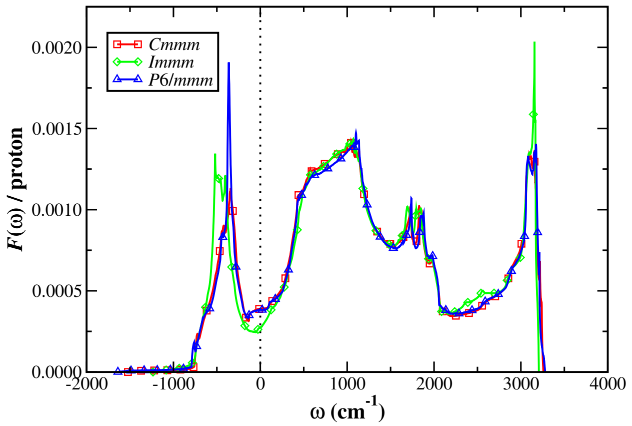


SUPPLEMENTARY FIG. 5. $F(\omega)$ of the candidate (atomic) structures, at 200 GPa. The dotted line is used to separate the stable from unstable (imaginary) phonon frequencies.

## TABLES

SUPPLEMENTARY TABLE I. Lattice parameters of the body-centered tetragonal (BCT) structures of atomic metallic hydrogen. All parameters are reported in the $I4_1/amd$ space-group representation; with two symmetry-inequivalent atoms, at the fractional coordinates (0.000 0.750 0.125) and (0.000 0.250 0.875).

| Structure | Pressure (GPa) | Lattice Parameters (Å) |
|---|---|---|
| $c/a \ll 1$ | 0 | $a = 5.95685$ $c = 0.98999$ |
| $\beta$-Sn | 350 | $a = 1.79839$ $c = 1.63959$ |
| diamond | 100 | $a = 1.42884$ $c = 2.02069$ |
| Cs-IV | 250 | $a = 1.37369$ $c = 3.15838$ |

| | | |
|---|---|---|
| $c/a \gg 1$ | 500 | $a = 0.99235$ $c = 4.61180$ |

SUPPLEMENTARY TABLE II. Structural parameters of the candidate mixed atomic/molecular structures of metastable metallic hydrogen, at 0 GPa (Supplementary Fig. 2). Only the fractional coordinates of symmetry-inequivalent atoms are reported.

| Space Group No. Atoms | Lattice Parameters (Å, °) | | | Atomic Coordinates (fractional) | | | |
|---|---|---|---|---|---|---|---|
| C2 | $a = 2.97050$ | $b = 5.98130$ | $c = 5.70570$ | H | 0.66669 | 0.36778 | 0.50002 |
| 10 | $\alpha = 90.00000$ | $\beta = 94.52530$ | $\gamma = 90.00000$ | H | 0.33331 | 0.36778 | 0.49998 |
| | | | | H | 0.91163 | 0.12167 | 0.04351 |
| | | | | H | 0.08837 | 0.12167 | 0.95649 |
| | | | | H | 0.00000 | 0.36798 | 0.50000 |
| C2/m | $a = 9.76920$ | $b = 5.60720$ | $c = 2.97540$ | H | 0.80711 | 0.50000 | 0.19903 |
| 14 | $\alpha = 90.00000$ | $\beta = 90.42510$ | $\gamma = 90.00000$ | H | 0.19289 | 0.50000 | 0.80097 |
| | | | | H | 0.86230 | 0.50000 | 0.02487 |
| | | | | H | 0.13770 | 0.50000 | 0.97513 |
| | | | | H | 0.00000 | 0.00000 | 0.00000 |
| | | | | H | 0.49997 | 0.50000 | 0.66680 |
| | | | | H | 0.50003 | 0.50000 | 0.33320 |
| Pm | $a = 2.98060$ | $b = 5.67400$ | $c = 6.00660$ | H | 0.56933 | 0.50000 | 0.12000 |
| 9 | $\alpha = 90.00000$ | $\beta = 91.32030$ | $\gamma = 90.00000$ | H | 0.24188 | 0.00000 | 0.89333 |
| | | | | H | 0.12409 | 0.00000 | 0.43782 |
| | | | | H | 0.75307 | 0.50000 | 0.20762 |
| | | | | H | 0.29284 | 0.00000 | 0.34697 |
| | | | | H | 0.90870 | 0.00000 | 0.89316 |
| | | | | H | 0.22800 | 0.50000 | 0.62531 |
| | | | | H | 0.57514 | 0.00000 | 0.89335 |
| | | | | H | 0.05381 | 0.50000 | 0.71362 |

SUPPLEMENTARY TABLE III. Structural parameters of the candidate (atomic) structures, at 0 GPa (Fig. 4 in the main text). Only the fractional coordinates of symmetry-inequivalent atoms are reported.

| Space Group<br>No. Atoms | Lattice Parameters<br>(Å, °) | | | Atomic Coordinates<br>(fractional) | | | |
|---|---|---|---|---|---|---|---|
| Pmmm | $a = 0.99120$ | $b = 2.62540$ | $c = 3.21100$ | H | 0.00000 | 0.50000 | 0.50000 |
| 1 | $\alpha = 90.00000$ | $\beta = 90.00000$ | $\gamma = 90.00000$ | | | | |
| Cmmm | $a = 3.67880$ | $b = 4.27280$ | $c = 0.99160$ | H | 0.50000 | 0.00000 | 0.00000 |
| 2 | $\alpha = 90.00000$ | $\beta = 90.00000$ | $\gamma = 90.00000$ | | | | |
| Immm | $a = 2.94940$ | $b = 4.84180$ | $c = 0.99130$ | H | 0.50000 | 0.00000 | 0.00000 |
| 2 | $\alpha = 90.00000$ | $\beta = 90.00000$ | $\gamma = 90.00000$ | | | | |
| P6/mmm | $a = 2.88110$ | $b = 2.88110$ | $c = 0.99160$ | H | 0.00000 | 0.00000 | 0.50000 |
| 1 | $\alpha = 90.00000$ | $\beta = 90.00000$ | $\gamma = 120.00000$ | | | | |

SUPPLEMENTARY TABLE IV: Structural parameters of the relaxed supercells (2×2×2) of the candidate (atomic) structures, at 0 GPa (Supplementary Fig. 4). Only the fractional coordinates of symmetry-inequivalent atoms are reported.

| Space Group<br>No. Atoms | Lattice Parameters<br>(Å, °) | | | Atomic Coordinates<br>(fractional) | | | |
|---|---|---|---|---|---|---|---|
| Pmmm | $a = 2.80470$ | $b = 6.02640$ | $c = 6.21130$ | H | 0.63413 | 0.50000 | 0.50000 |
| 8 | $\alpha = 90.00000$ | $\beta = 90.00000$ | $\gamma = 90.00000$ | H | 0.36587 | 0.50000 | 0.50000 |
| | | | | H | 0.86598 | 0.50000 | 0.00000 |
| | | | | H | 0.13402 | 0.50000 | 0.00000 |
| | | | | H | 0.86595 | 0.00000 | 0.50000 |
| | | | | H | 0.13405 | 0.00000 | 0.50000 |
| | | | | H | 0.86603 | 0.00000 | 0.00000 |
| | | | | H | 0.13397 | 0.00000 | 0.00000 |
| P2/m | $a = 7.45230$ | $b = 2.81320$ | $c = 9.40380$ | H | 0.50000 | 0.63372 | 0.00000 |
| 16 | $\alpha = 90.00000$ | $\beta = 90.05420$ | $\gamma = 90.00000$ | H | 0.50000 | 0.36628 | 0.00000 |
| | | | | H | 0.73972 | 0.86632 | 0.26047 |

| | | | | | | | |
|---|---|---|---|---|---|---|---|
| | | | | H | 0.26028 | 0.86632 | 0.73953 |
| | | | | H | 0.26028 | 0.13368 | 0.73953 |
| | | | | H | 0.73972 | 0.13368 | 0.26047 |
| | | | | H | 0.50000 | 0.63367 | 0.50000 |
| | | | | H | 0.50000 | 0.36633 | 0.50000 |
| | | | | H | 0.73974 | 0.86634 | 0.73955 |
| | | | | H | 0.26026 | 0.86634 | 0.26045 |
| | | | | H | 0.26026 | 0.13366 | 0.26045 |
| | | | | H | 0.73974 | 0.13366 | 0.73955 |
| | | | | H | 0.00000 | 0.86639 | 0.00000 |
| | | | | H | 0.00000 | 0.13361 | 0.00000 |
| | | | | H | 0.00000 | 0.63369 | 0.50000 |
| | | | | H | 0.00000 | 0.36631 | 0.50000 |
| $P\bar{1}$ | $a = 2.83260$ | $b = 6.41830$ | $c = 10.32420$ | H | 0.32514 | 0.11451 | 0.34815 |
| 16 | $\alpha = 90.42390$ | $\beta = 90.13890$ | $\gamma = 90.42460$ | H | 0.67486 | 0.88549 | 0.65185 |
| | | | | H | 0.80202 | 0.82474 | 0.13081 |
| | | | | H | 0.19798 | 0.17526 | 0.86919 |
| | | | | H | 0.17144 | 0.14489 | 0.40424 |
| | | | | H | 0.82856 | 0.85511 | 0.59576 |
| | | | | H | 0.67449 | 0.92442 | 0.11744 |
| | | | | H | 0.32551 | 0.07558 | 0.88256 |
| | | | | H | 0.15201 | 0.67680 | 0.36627 |
| | | | | H | 0.84799 | 0.32320 | 0.63373 |
| | | | | H | 0.82001 | 0.38189 | 0.15432 |
| | | | | H | 0.17999 | 0.61811 | 0.84568 |
| | | | | H | 0.28642 | 0.57918 | 0.38045 |
| | | | | H | 0.71358 | 0.42082 | 0.61955 |
| | | | | H | 0.66651 | 0.36213 | 0.09607 |
| | | | | H | 0.33349 | 0.63787 | 0.90393 |
| P2/m | $a = 6.26960$ | $b = 2.79940$ | $c = 6.28350$ | H | 0.00000 | 0.13425 | 0.00000 |

| | | | | | | | |
|---|---|---|---|---|---|---|---|
| 8 | $\alpha = 90.00000$ | $\beta = 119.42060$ | $\gamma = 90.00000$ | H | 0.00000 | 0.86575 | 0.00000 |
| | | | | H | 0.50000 | 0.13427 | 0.50000 |
| | | | | H | 0.50000 | 0.86573 | 0.50000 |
| | | | | H | 0.50000 | 0.13424 | 0.00000 |
| | | | | H | 0.50000 | 0.86576 | 0.00000 |
| | | | | H | 0.00000 | 0.36564 | 0.50000 |
| | | | | H | 0.00000 | 0.63436 | 0.50000 |
